# Supplementary material for: Fractional charges in conventional sequential electron tunneling
Source: arXiv:1811.06468 ancillary file (2019-06-19)
Supplement: Supplementary file 1 [file suppl_fractional_charges_RR.pdf]

# Supplemental Material: Fractional charges in conventional sequential electron tunneling

Roman-Pascal Riwar[1]

[1]*JARA Institute for Quantum Information (PGI-11), Forschungszentrum Jülich, 52425 Jülich, Germany*

## S1 Model Hamiltonians for the quantum dot systems

In the main text, we consider two simple transport models, the single-level quantum dot and the serial double quantum dot, both coupled to normal metal reservoirs. For the sake of completeness, we here provide the Hamiltonians of these models.

### S1.1 The single-level quantum dot

The single-level quantum dot, depicted in Fig. 2 in the main text, can be described by the Hamiltonian

$$H = H_{\mathrm{QD}} + H_{\mathrm{T}} + \sum_{\alpha=\mathrm{L,R}} H_{\alpha}, \tag{S1}$$

where the Hamiltonian $H_{\mathrm{QD}}$ describes the single-level dot itself

$$H_{\mathrm{QD}} = \sum_{s} \epsilon d_s^{\dagger} d_s + U \frac{n\left(n-1\right)}{2} \tag{S2}$$

where $d_s^{(\dagger)}$ annihilates (creates) an electron with spin $s$ and energy $\epsilon$ in the dot, and $n = \sum_s d_s^{\dagger} d_s$ is the dot electron number. The parameter $U$ characterizes the onsite Coulomb interaction. We henceforth set it to $U \to \infty$, thus disregarding the possibility of an occupation number greater than 1. The spin degeneracy is $\sigma = \sum_s$. For an ordinary system of spin 1/2 electrons, $\sigma = 2$. The reservoir Hamiltonians are given as

$$H_{\alpha} = \sum_{ks} \left(\epsilon_k - \mu_{\alpha}\right) c_{\alpha k s}^{\dagger} c_{\alpha k s}, \tag{S3}$$

where $c_{\alpha k s}^{(\dagger)}$ annihilates (creates) an electron with spin $s$, momentum $k$ and energy $\epsilon_k$ in reservoir $\alpha$. Finally, the tunnel Hamiltonian characterizes the electron transport between dot and reservoirs. It can be given as

$$H_{\mathrm{T}} = \sum_{\alpha k s} \gamma_{\alpha k} c_{\alpha k s}^{\dagger} d_s + \mathrm{h.c.}, \tag{S4}$$

where $\gamma_{\alpha k}$ describes the tunneling amplitudes. The transition rates in Eq. (10) can be computed from above Hamiltonian through standard Fermi golden rule. For a derivation of the transition rates, see Ref. [79]. In the wideband limit, $\gamma_{\alpha k} = \gamma_{\alpha}$, one finds the tunneling rates $\Gamma_{\alpha} = 2\pi\gamma_{\alpha}^2\rho$, where $\rho$ is the density of states of the reservoir at the Fermi level.

### S1.2 The serial double quantum dot

The double quantum dot, as shown in Fig. 4, is described by the following Hamiltonian

$$H = H_{\mathrm{QDL}} + H_{\mathrm{QDR}} + H_{\mathrm{L}\leftrightarrow\mathrm{R}} + \sum_{\alpha} H_{\mathrm{T}\alpha} + \sum_{\alpha} H_{\alpha}. \tag{S5}$$

Here, there are now left and right quantum dots, each described by

$$H_{\mathrm{QD}\alpha} = \sum_{s} \epsilon_{\alpha} d_{\alpha s}^{\dagger} d_{\alpha s} + U \frac{n_{\alpha}\left(n_{\alpha}-1\right)}{2}, \tag{S6}$$

where the electron annihilation (creation) operators for the left and right dot are respectively denoted as $d_{\alpha s}^{(\dagger)}$, and $n_\alpha = \sum_s d_{\alpha s}^\dagger d_{\alpha s}$. We allow for the two quantum dot energies $\epsilon_\alpha$ to be different, while still $U \to \infty$. The reservoir Hamiltonians are unchanged, and are still given by Eq. (S3). The tunneling between left and right dot and the corresponding reservoirs is now described through

$$H_{\mathrm{T}\alpha} = \sum_{\alpha k s} \gamma_{\alpha k} c_{\alpha k s}^\dagger d_{\alpha s} + \text{h.c.} \tag{S7}$$

We are left with providing the Hamiltonian $H_{\mathrm{L}\leftrightarrow\mathrm{R}}$ which describes the coupling between the two dots. We include both a capacitive and a tunnel coupling,

$$H_{\mathrm{L}\leftrightarrow\mathrm{R}} = H_C + H_{\mathrm{T,L}\leftrightarrow\mathrm{R}} \tag{S8}$$

The capacitive coupling is

$$H_C = U_{\mathrm{LR}} n_{\mathrm{L}} n_{\mathrm{R}}. \tag{S9}$$

We likewise set $U_{\mathrm{LR}} \to \infty$, such that there can be only one extra electron in the entire double quantum dot system. As for the tunnel coupling, we write it as

$$H_{\mathrm{T,L}\leftrightarrow\mathrm{R}} = \left( \sum_s \left[ \delta_{\mathrm{LR}} + \sum_q \lambda_q \left( a_q^\dagger + a_{-q} \right) \right] d_{\mathrm{L}s}^\dagger d_{\mathrm{R}s} + \text{h.c.} \right) + \sum_q \omega_q a_q^\dagger a_q.$$

In general, the electron exchange between the two quantum dots can be coherent, described by the first term $\delta_{\mathrm{LR}}$, or can be mediated through an inelastic process. We here include the possibility for electron tunneling mediated via phonons with frequency $\omega_q$ for wave vector $q$, annihilated (created) through $a_q^{(\dagger)}$. Such an interaction is described e.g. in Ref. [83]. We assume in Sec. **??**, that the inelastic process dominates over the coherent interdot tunneling. The validity of this assumption depends of course on the details of the double quantum dot. However, one can argue that it is always possible to sufficiently detune the two quantum dot levels, such that the coherent, elastic term is suppressed, and the dominant process is given by inelastic tunneling, see also Ref. [82].

We can now likewise perform a Fermi golden rule calculation to arrive at the inelastic interdot transition rates, as introduced in Eq. (19).

Note that the electron-phonon interaction in general also couples to the single dot levels in $H_{\mathrm{QD}\alpha}$ [83]. This does however not provide any relevant physics: it results in a renormalization of the single-level energy, which we can ignore for large detuning, and a dephasing process, which is irrelevant as we do not consider coherent states. This is why we discard this additional interaction.

## S2 Derivation of $\mathbb{Z}_2$-number from nonequilibrium geometric phase

In the main text, we argue that the geometric phase defined in the counting field gives rise to a topological number depending on the periodicity of the eigenspectrum of $W$, see Eq. (30). We here show, how this relation is derived.

### S2.1 Exceptional points for complex counting fields

The first step involves extending our considerations to complex counting fields, whereby we replace $e^{i\chi} \to z \in \mathbb{C}$ and $e^{-i\chi} \to 1/z$, such that the real counting field corresponds to the unit circle $|z| = 1$. That is, the discreteness of the process is now captured in the fact that $W(z) = W(\chi)|_{e^{i\chi}\to z}$ can be written in terms of a Laurent series, $W(z) = \sum_N z^N W_N$. While this is first and foremost a formal step for the demonstration of Eq. (30), we stress that complex counting fields have also physical meaning. Most importantly, complex extensions of the counting field are important for capturing microreversibility as we will mention again later. Moreover, we emphasize that the eigenspectrum of $W(z)$ for a general complex $z$ is in fact itself experimentally measurable by means of waiting time distributions. Finally we note that also the study of dynamical phase transition by means of Lee-Yang zeros relies likewise on the notion of complex counting fields [25, 59].

With the generalization to complex fields, each element in $W(z)$ is in general analytic for all $z$, except at $z = 0$ and $z = \infty$. Therefore, the coefficients in the characteristic polynomial to determine the eigenvalues, $\det[W(z) - \lambda]$, are

also analytic for finite $z$. This will turn out to be important for our subsequent discussion of both the eigenspectrum as well as geometric phases occuring in a parallel vector transport.

We assume, for the sake of simplicity, that the eigenspectrum of $W(z)$ for $|z| = 1$, that is, for *real* counting fields $\chi$, is nondegenerate, and can be decomposed into left and right eigenvectors. Importantly, we observe that even with this assumption, two eigenvalues of $W(z)$ can be degenerate for *complex* $z$. This can however occur only in isolated points - so-called exceptional points. This is simply so because for a complex spectrum, the degeneracy of two eigenvalues $\lambda_{n_1}(z) = \lambda_{n_2}(z)$ provides one complex condition, which can be met by the one independent complex variable $z$. Given the point $z_0$, where the two eigenvalues $n_1$ and $n_2$ meet, we can now explore its neighbourhood, $z = z_0 + \delta z$. By expanding the characteristic polynomial $\det[W(z) - \lambda]$ in lowest orders in $\delta z$, and using the analyticity of $W(z)$, it is straightforward to show that the two eigenvalues taking part in the degeneracy behave locally as $\lambda_{n_1,n_2}(z) = \widetilde{\lambda}^{(0)} \pm \widetilde{\lambda}^{(1/2)}\sqrt{\delta z} + \mathcal{O}[\delta r]$ where $\widetilde{\lambda}^{(0)}$ and $\widetilde{\lambda}^{(1/2)}$ are complex numbers. The other (nondegenerate) eigenvalues on the other hand behave simply as $\lambda_{n\neq n_{1,2}}(z) = \widetilde{\lambda}^{(0)}_n \pm \widetilde{\lambda}^{(1)}_n \delta z + \mathcal{O}[\delta r^2]$. The degenerate subpart of the spectrum therefore inherits the behaviour of the complex square root function; if we require the spectrum to be continuous, the function becomes multivalued. We will for the sake of simplicity resort from now on to contours parametrized as $z = z_0 + \delta r e^{i\theta}$, such that the eigenspectrum becomes $\lambda_{n_1,n_2}(z) \approx \widetilde{\lambda}^{(0)} \pm \widetilde{\lambda}^{(1/2)}\sqrt{\delta r}e^{i\theta/2}$ which is thus continuous, but $4\pi$-periodic. Consequently, circumventing the exceptional point provides a braiding of the eigenvalues $n_1$ and $n_2$. We have to circle it twice in order to map the spectrum onto itself, see Fig. S1.

Based on the above we can make a very direct link to the standard braid theory. Namely, to each exceptional point we can assign a generator of the braid group $\sigma_n$. As a reminder, in braid theory [77], the generator $\sigma_n$ is a representation of the operation that braids two strands $n-1$ and $n$. In analogy, in the present case here, we may assign a generator $\sigma_n$ to an exceptional point that braids eigenvalues $\lambda_n$ and $\lambda_{n-1}$, see Fig. S1.

Having established this formal framework, we can introduce the notion of a topological conservation law, which concerns the chirality of the braids. Namely, we notice that for finite $z$, we only get exceptional points of the form $\widetilde{\lambda}^{(0)} \pm \widetilde{\lambda}^{(1/2)}\sqrt{\delta z}$, that is, once we defined the orientation of our manifold $z$, the eigenvalues braid around each other with a given chirality. Globally, there must however be a conservation law of braid generators, that is, to every exceptional point with a generator $\sigma_n$, there must somewhere be a corresponding generator $\sigma_n^{-1}$, which braids with the opposite chirality. This is due to the fact, that we can always find some closed path in $z$ which does not contain any exceptional points. Along this path, the spectrum is necessarily trivial, and that means that both on the inside and outside of this path, the total braid must be trivial, leading necessarily to the presence of a total conservation law. Since we now know that for finite $z$, the degeneracies must be of the form $\widetilde{\lambda}^{(0)} \pm \widetilde{\lambda}^{(1/2)}\sqrt{\delta z}$, they cannot be of the inverse form $\sigma_n^{-1}$. We thus have to conclude that the inverse braids can only be located at the poles $z = 0$ and $z = \infty$, where $W(z)$ is nonanalytic.

We can see this fact for instance in the vicinity of $z = 0$. Here, the Laurent terms $W_N$ with negative power $N < 0$ become important. If those terms are nonzero, the eigenvalues close to $z$ that are not involved in a braiding, in general diverge as $\sim 1/z$, while eigenvalues that are braided at $z = 0$ diverge as $\sim 1/\sqrt{z}$ (or lower fractal powers, when more than one generator coincide at this pole). Curiously, even though the eigenvalues diverge when approaching $z \to 0$, they can be considered as degenerate in the sense that they diverge with a power less than $z^{-1}$. They therefore correspond likewise to exceptional points. As these braids are of the form $\sim 1/\sqrt{z}$, it is obvious that they have indeed the opposite braiding chirality. The $z = \infty$ case can be treated similarly, when performing the mapping $W(z) \to W(1/z)$, i.e., inverting the direction of the detector, such that events that increase (decrease) the detector state now decrease (increase) them. With this map, generators originally "located" at $z \to \infty$ are now found at $z = 0$.

In Fig. S2, we see generic sketches of what we can expect the spectrum in $z$-space to look like in general. The exceptional points (black dots) each have assigned to them a braid generator. The solid curves connect two exceptional points with opposing braid chirality, with the inverse generators located at the two poles $z \to 0$ and $z \to \infty$, respecting the global conservation law. Let us stress at this point that the depiction of the inverse generators for $z \to \infty$ at specific points on the $\infty$-line in Fig. S2 is just done for purposes of visualization; these inverse generators to not actually have a well-defined location at $z \to \infty$. As we mentioned before, the most tangible way to visualise these generators is through the map $W(z) \to W(1/z)$, where these inverse generators occur now at $z = 0$.

The connecting curves can be though of as linking the two braid generators that are pair-wise created (annihilated) when smoothly turning on (off) the counting field, say for some continuous map $W(z, r)$, such that, e.g., $W(z, 0) = W(1)$, where the spectrum is necessarily and obviously trivial, and $W(z, 1) = W(z)$. In this context, we define continuous in the sense that the creation of braid generator pairs is such that the $\sigma_n$ change their position in $z$ continuously as a function of $s$. We can conclude that the poles at $z \to 0, \infty$ act in some sense as a place of origin for the braid generators. When switching on the counting field, $r = 0 \to r = 1$, a $\sigma_n$ and $\sigma_n^{-1}$ pair get created either at $z \to 0$, or at $z \to \infty$. For increasing $r$, the generator $\sigma_n$ is then dragged into the area of finite $z$, while the $\sigma_n^{-1}$ stay fixed at the respective poles. Thus, if we imagine such a transition from a $W(z, 0)$ with a trivial spectrum for all $z$, to a generally braided spectrum for $W(z, 1)$, we can think of each of the two poles with their collection of generator

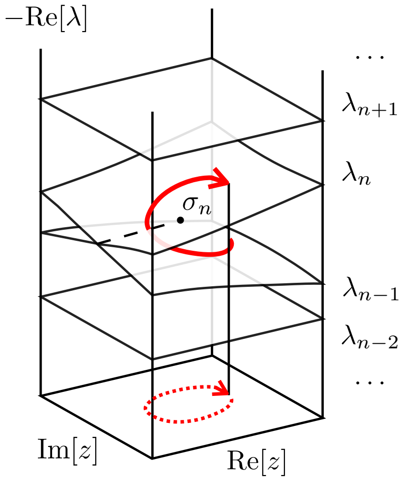


FIG. S1. The spectrum of $W(z)$ in the neighbourhood of an exceptional point braiding $\lambda_{n-1}$ and $\lambda_n$. Circumventing the exceptional point provides a lift from one to the other eigenvalue, such that we can assign a braid generator $\sigma_n$ to the degeneracy.

pairs like a network with a single node, where all the inverse generators are located, see also Fig. S2.

We can add one more detail regarding the nature of the poles, which becomes important later. It is related to the already mentioned fact, that when approaching $z \to 0$ ($z \to \infty$), the components $W_N$ of the Laurent series with positive (negative) powers, $N > 0$ ($N < 0$) become insignificant. In order to describe the spectrum of the 0-pole, it suffices therefore to consider the matrix $W_<(z) = \sum_{N\leq 0} z^N W_N$, or for the $\infty$-pole, the matrix $W_>(z) = \sum_{N\geq 0} z^N W_N$. On the one hand side, we can thus state that the topology in the vicinity of $z \to 0$ ($z \to \infty$) is exclusively determined by the processes that decrease (increase) the detector state. On the other hand, looking at the spectrum of $W_<(z)$ for $z \to \infty$ (or likewise the spectrum of $W_>$ for $z \to 0$), we find essentially the spectrum of $W_0$ which is generically trivial. This second observation will be handy in order to separately annihilate, or "collapse", the network emerging from either the 0-pole or the $\infty$-pole, while retaining the other, through the defining some appropriate map, $W(z,s)$, such that $W(z,0) = W_{\lessgtr}(z)$ and $W(z,1) = W(z)$, which is going to be needed in Sec. S2 S2.4.

The connecting curves between generators $\sigma_n$ and their inverses $\sigma_n^{-1}$ can actually be explicitly visualized, by projecting the complex spectrum on one axis, $\bar{\lambda}_n(z) = \mathrm{Re}\left[e^{i\varphi}\lambda_n(z)\right]$ (such that, e.g., $\varphi = 0$ corresponds to a projection on the real axis), and plotting the degeneracies of the *projected* spectrum as a function of $z$. Two generators with opposite braid will be connected by a degeneracy curve. These curves will change their path for a different values of $\varphi$, while the end points, corresponding to the exceptional points, remain fixed. In Fig. S2 we refrained from an explicit calculation of these lines, because the connecting curves may take rather peculiar, nontrivial shapes that make it difficult to interpret them. Consequently, in Fig. S2 the connecting curves are merely sketches, aimed to guide the eye.

Overall, we can state, that to every exceptional point for finite $z$, with a generator $\sigma_n$, we must find an inverse generator $\sigma_n^{-1}$, located either at the $z \to 0$ or the $z \to \infty$ pole. These pairs of generators are connected through a curve. In order to figure out the braid of a spectrum on a closed path on $z$, we add the corresponding generator when the path intersects the connecting curve.

To summarize, we now understand on a much deeper level the braiding of the FCS spectrum at $|z| = 1$, that is for real counting fields. Namely, its topology can be derived by an extension to complex counting fields, and analyzing the exceptional points (degeneracies) in the complex space. We may then assign the corresponding braid generator for each exceptional point, and trace the connecting curves between each pair of generator and inverse. Finally, for each connecting curve that crosses the unit circle $|z| = 1$, we can add the corresponding generator to determine the braid of the eigenspectrum for real counting fields, i.e., at $|z| = 1$.

In fact, we can therefore loosely think of this as a version of a bulk-edge correspondence: the exceptional points and their corresponding generators *inside* the unit circle (bulk), provide the braiding topology of the spectrum *at* the unit circle $|z| = 1$ (edge).

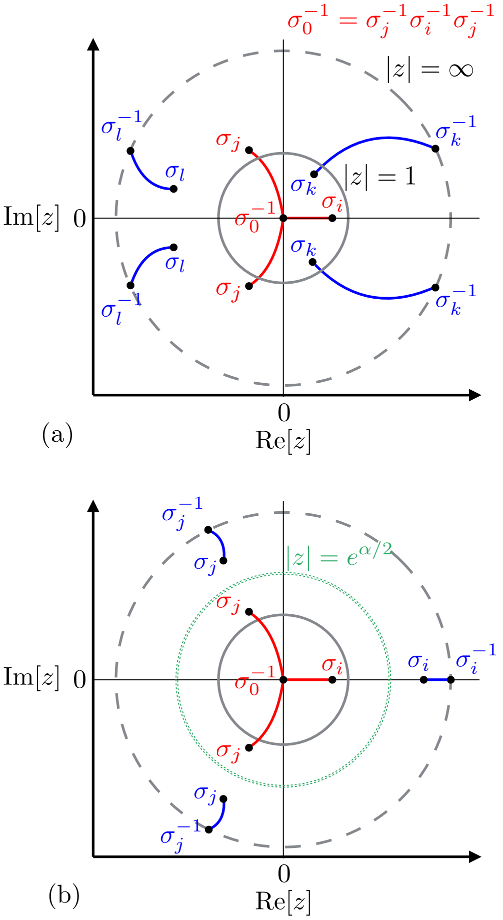


FIG. S2. Possible configurations of exceptional points in the complex counting field $z$. To each exceptional point, we may assign a generator of the braid group, $\sigma_i$. The inverse generators $\sigma_i^{-1}$ are located at the two poles, either $z = 0$ or $z = \infty$. In (a) we show the generic case of a matrix with the symmetry $W^*(z) = W(z^*)$ (Markov chain). All exceptional points that do not lie on the real axis have a complex conjugate counterpart. In (b), there is in addition microreversibility, $W^T(z) = W(e^\alpha/z)$, such that the generators inside and outside the symmetry "axis" $|z| = e^{\alpha/2}$ (marked in green) appear mirrored.

### S2.2 Importance of symmetries

Importantly, as we show now, the explicit configuration of exceptional points is sensitive to symmetries. However, as we will argue at the end of this section, none the symmetries inhibit the observation of a braided eigenspectrum with broken periodicity.

There are two main symmetries for $W$. Firstly, we have initially assumed that the system dynamics is represented as a Markov chain, where all transition rates are real. In the presence of the counting field, this results in the symmetry $W^*(z) = W(z^*)$, and as a consequence, each exceptional point at some $z = z_0$ has a counterpart at $z = z_0^*$ with the same generator, see Fig. S2a.

Secondly, microreversibility represents a fundamental symmetry for open systems. Most notably, it was shown that microreversibility establishes a symmetry in the full-counting statistics that allows a generalization of fluctuation relations to nonequilibrium [? ? ]. In the most general case, this symmetry can be formulated only when taking into account the statistics of heat currents in addition to particle currents. This is clearly outside the scope of the present paper, and will be delegated to future research. However, a simple version exists under the assumption that the temperature in both reservoirs is equal. Then,

$$W^T(z) = W(e^\alpha/z) \tag{S10}$$

where $\alpha = (\mu_R - \mu_L)/k_B T$ captures the bias in the chemical potential. As a consequence, and similar to before, we find that if there is an exceptional point at some $z = z_0$, there must be one at $z = e^\alpha/z_0$, again with the same

braiding generator, see Fig. S2b. Thus microreversibility restricts the topology of $W(z)$ to some extent. We further note that the circle $|z| = e^{\alpha/2}$ corresponds to a symmetry "axis". The spectrum of $W(z)$ for $|z| = e^{\alpha/2}$ is consequently trivial. This is a generalisation of the observation of Ren et al. [6]. They found that in equilibrium, the spectrum of $W(z)$ at $|z| = 1$ must be trivial, which agrees with our conclusion, since equilibrium requires $\alpha = 0$. For finite $\alpha$, this symmetry "axis" with a trivial spectrum gets either pushed inwards or outwards, depending on the sign of $\alpha$, allowing for a nontrivial spectrum for $|z| = 1$.

Importantly, we can conclude that apart from the very explicit case of equilibrium transport, none of the above symmetries render the observation of a braided spectrum at $|z| = 1$ impossible. They merely limit the degrees of freedom for the position of the exceptional points.

### S2.3 Topology for special Hermitian matrices

Finally, we want to comment on a particularity for matrices that are Hermitian for $|z| = 1$. In fact, matrices that describe incoherent transport become Hermitian in equilibrium, $\alpha = 0$, where they are in general trivial [6]. However, in Sec. III we treated very special Hermitian matrices, which describe the transport of coherent Cooper pair transport in topological superconducting junctions. Here, *additional* symmetries yet again enforce a topological transition even in the Hermitian case. These phases can likewise be understood in terms of exceptional points in the complex plane.

To this end, we again follow the same strategy, namely to generalize $H(\phi)$ to complex $\phi$, by means of decomposing $H(\phi) = \sum_N e^{iN\phi} H_N$, and replacing $e^{i\phi} \to z$. Here, in order for a periodicity breaking to occur for a Hermitian matrix with a real spectrum, two exceptional points - to each of which we assign the generator $\sigma_n$ - need to approach each other and finally meet a single point on $|z| = 1$, resulting in a regular degeneracy which behaves locally as $\sim \pm\delta z$ (instead of $\sim \pm\sqrt{\delta z}$). For a general matrix $H$, this merging of exceptional points is not stable. In fact, the meeting of two exceptional points on the real line corresponds to an additional condition on the eigenspectrum. Any small arbitrary change of the matrix $H$ can lead to a violation of this extra condition, and make the spectrum trivial. The special symmetries that are present in the Hamiltonians for the topological superconducting junctions (as we introduce them in Sec. III) on the other hand provide the necessary extra condition, and thus stabilize this merger of exceptional points. This establishes in yet another way the relation between Hermitian matrices with broken periodicities and the more general case of non-Hermitian matrices in terms of degeneracies in the space of complex $\phi$ (or $\chi$). We note that the only difference is that the assignment of a braid generator at this merger point is impossible, see Fig. S3 and caption.

### S2.4 A $\mathbb{Z}_2$ topological invariant emerging from geometric phases

As indicated in the main text, when considering time-dependent counting fields, a response in form of a geometric phase emerges, in analogy to the Berry phase. Here, we show how Eq. (30) can be demonstrated, that is, how the geometric phase gives rise to a $\mathbb{Z}_2$-number. As we will see now, for this purpose, the introduction of complex counting fields, $e^{i\chi} \to z$, from the previous sections, and the understanding of the braided spectrum in terms of exceptional points in the complex plane is indispensable.

As in the main text, we introduce a time-dependent complex counting field $z \to z(t)$. In an adiabatic expansion of the time evolution of $|P(t))$, $\partial_t |P(t)) = W[z(t)] |P(t))$, there occurs the adiabatic response function

$$a_n(t_0) = e^{-\int_0^{t_0} dt (n[z(t)]|\partial_t|n[z(t)])} (n[z(t_0)]|n[z(0)]) \tag{S11}$$

along the same lines as Eq. (37) in Sec. IV C. We rewrite this function as $a_n[\mathcal{C}] = \mathcal{B}_n[\mathcal{C}] (n(z_f)|n(z_i))$ with the generalised geometric phase

$$\mathcal{B}_n[\mathcal{C}] = e^{-\int_{\mathcal{C}} dz (n(z)|\partial_z|n(z))} \tag{S12}$$

where the time-dependent driving $z(t)$ is represented as the contour $\mathcal{C}$ in the complex plane, with starting and ending points $z_i = z(0)$ and $z_f = z(t_0)$, respectively.

The function $a_n[\mathcal{C}]$ is manifestly gauge invariant, as we may multiply the eigenvectors with an arbitrary, invertible, differentiable complex function $|n(z)) \to \gamma(z) |n(z))$, $(n(z)| \to \frac{1}{\gamma(z)} (n(z)|$ , and $a$ remains unchanged. If we are able to find a contour, such that the system at $z_f$ returns to its initial vector at $z_i$, and if we are able to find an appropriate gauge, then $(n(z_f)|n(z_i)) = 1$, and $\mathcal{B}_n[\mathcal{C}]$ and $a_n[\mathcal{C}]$ are equivalent, and can be used interchangeably - or in other words, for a closed contour, we may measure $a_n$ in order extract the geometric phase. As for the contours, this requires that we consider closed paths in $z$, which we denote as $\mathcal{C}_\circ$. Importantly, in the presence of braiding, it

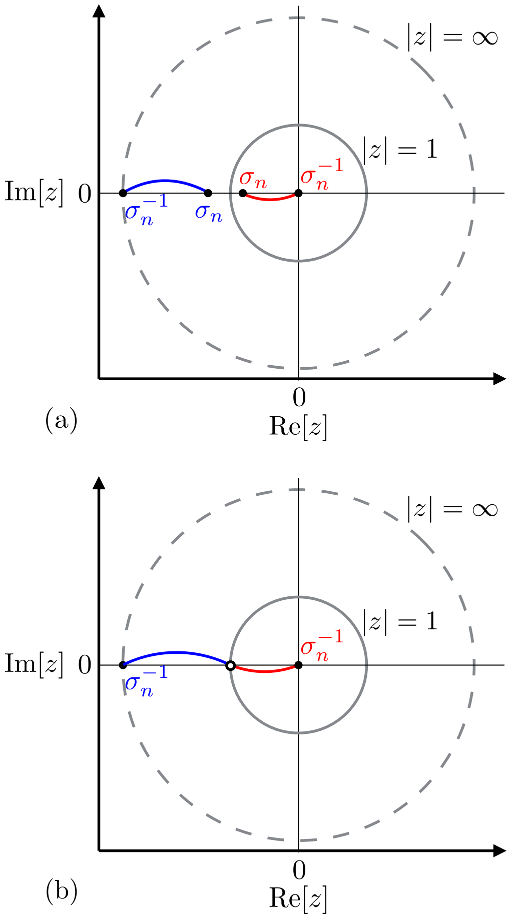


FIG. S3. Merging of exceptional points for special Hermitian matrices, that is, with a spectrum that is real on the unit circle, $|z| = 1$. We consider the case of either a trivial spectrum (a) or a real spectrum with broken periodicity (b). The former depicts the ordinary case, where the two degenerate eigenvalues behave as $\sim \pm\sqrt{\delta z}$, where as in (b), the two regular exceptional points merge into a new degeneracy of the form $\sim \pm\delta z$. In the latter case, we can no longer assign a braid generator to the spectrum for $|z| = 1$. This can be understood as follows. If we were to choose to consider the path $|z| < 1$, the spectrum on this path can be described by the generator $\sigma_n^{-1}$, while for $|z| > 1$ the spectrum corresponds to $\sigma_n$. Right at the transition of these two paths, $|z| = 1$, the braid is ill-defined.

does not suffice in general, that the contour is closed, but we have to supplement the contour with multiple windings in order to return to the original eigenvector, in accordance of an eigenspectrum with broken periodicity. Naturally, this means that it does not suffice in general to consider only one individual band, but all bands need to be taken into account. We therefore consider the quantity

$$\mathcal{Z}_{\mathcal{C}_\circ} = \prod_\nu a_\nu \left[\mathcal{C}_\circ\left(p_\nu\right)\right] \tag{S13}$$

making use of the reduced band notation $\nu$ introduced in the main text, which is justified due to redundancy. We denote with $\mathcal{C}_\circ\left(p_\nu\right)$ the contour $\mathcal{C}_\circ$ with $p_\nu$ windings, i.e., $\mathcal{C}_\circ\left(1\right) = \mathcal{C}_\circ$. In order to prove that $\mathcal{Z}_{\mathcal{C}_\circ} = \pm 1$, depending on the braid of the spectrum, it turns out to be useful to express it in terms of the geometric phases $\mathcal{B}$. Therefore, we require that the eigenvectors are chosen in a gauge, such that the eigenvectors for $\nu$ have likewise the periodicity $p_\nu$, we may rewrite the above as

$$\mathcal{Z}_{\mathcal{C}_\circ} = \prod_\nu \mathcal{B}_\nu \left[\mathcal{C}_\circ\left(p_\nu\right)\right] = \exp\left[-\sum_\nu \oint_{\mathcal{C}_\circ\left(p_\nu\right)} dz \left(\nu\left(z\right)\right| \partial_z \left|\nu\left(z\right)\right)\right] \tag{S14}$$

In the second equality, we have transformed the quantity $\mathcal{Z}$ into the exponential of a sum of integrals over closed contours. That is, we have arrived at a formula, where we are able to apply the Cauchy integral theorem. In our

particular case, the theorem implies, that for contours that do not enclose any exceptional points, the integrals for each band are individually zero, making the geometric phase trivially equal 1. We may thus decompose the integral for any given contour into just a sum of small infinitesimal contours enclosing each an exceptional point at finite $z$ or the pole at $z = 0$. An example of such a decomposition into small contours is shown in Fig. S4. Our task therefore reduces now to finding the geometric phases for contours circling around these isolated exceptional points.

Let us therefore consider a closed contour enclosing an infinitesimally small area in $z$, that is, $z = z_0 + \delta z$. We first concentrate on $z_0$ being finite, that is, we exclude the pole at $z = 0$. We once more parametrize this closed contour in the simplest fashion as $z(\theta) = z_0 + \delta r e^{i\theta}$. When there are no exceptional points in the spectrum within this infinitesimal area, the eigenspectrum is analytic within this area, and we may likewise find an analytic representation of the eigenvectors which is $2\pi$-periodic in $\theta$. Consequently, we find in this trivial case that we return to the original eigenvector when we enclose the area just once, that is, for $\theta$ from 0 to $2\pi$, denoted as $\delta\mathcal{C}_\circ$, and find that $a_n[\delta\mathcal{C}_\circ] = 1$ as well as $\mathcal{B}_n[\delta\mathcal{C}_\circ] = 1$ for all $n$, in accordance with the Cauchy integral theorem.

If however the contour encloses an exceptional point which braids eigenvalues $n_1$ and $n_2$, then the spectrum for these two eigenvalues is approximately given by $\lambda_{n_1,n_2}(z) = \widetilde{\lambda}^{(0)} \pm \widetilde{\lambda}^{(1/2)} \sqrt{\delta r} e^{i\theta/2} + \mathcal{O}[\delta r]$, as pointed out previously. As a consequence, we can find a $4\pi$-periodic gauge where we can expand the two eigenvectors in this neighbourhood as

$$
\begin{aligned}
|n_{1,2}) &= \pm \frac{1}{\sqrt{\delta r}} e^{-i\theta/2} |\widetilde{n}) + |\partial\widetilde{n}) + \mathcal{O}\left[\sqrt{\delta r}\right] \\
(n_{1,2}| &= (\widetilde{n}| \pm \sqrt{\delta r} e^{i\theta/2} (\partial\widetilde{n}| + \mathcal{O}[\delta r] .
\end{aligned}
$$

We again change to the reduced notation for the braided band, $\nu_1$, such that $|\nu_1(\theta)) = |n_1(\theta))$ and $|\nu_1(\theta + 2\pi)) = |n_2(\theta))$ for $0 \leq \theta < 2\pi$. We note that the projector $|\nu_1)(\nu_1|$ contains a lowest order term with a square root divergence as $\delta r \to 0$. This means that at the exceptional point, the projector to this subspace is ill-defined (as is the definition of an exceptional point), and as a consequence, the function $(\nu(z)|\,\partial_z\,|\nu(z))$ is not analytic, and the contour integral nonzero.

As indicated above and in Fig. S1, after enclosing the exceptional point once we do not yet return to the same eigenvector, and thus, $a_{\nu_1}[\delta\mathcal{C}_\circ] = 0$. If we enclose the exceptional point twice, i.e. with a contour going from $\theta = 0$ to $4\pi$, denoted simply as $\delta\mathcal{C}_{2\circ}$, we return to the original eigenvalue and eigenvector, where we thus find a nonzero-geometric phase. Expanding the condition $(n_i\,|n_j) = \delta_{ij}$ up to zeroth order in $\delta z$, it follows that $(\widetilde{n}\,|\widetilde{n}) = 0$ and $(\widetilde{n}\,|\partial\widetilde{n}) = (\partial\widetilde{n}\,|\widetilde{n}) = 1/2$. Because of this, we find $a_{\nu_1}[\delta\mathcal{C}_{2\circ}] = \mathcal{B}_{\nu_1}[\delta\mathcal{C}_{2\circ}] = -1$. Since the remaining, trivial bands provide a zero geometric phase, we find

$$
\mathcal{Z}_{\delta\mathcal{C}_\circ} = \prod_\nu \mathcal{B}_\nu[\delta\mathcal{C}_{\circ,\nu}] = \prod_\nu a_\nu[\delta\mathcal{C}_{\circ,\nu}] = -1. \tag{S15}
$$

Here, $\delta\mathcal{C}_{\circ,\nu} = \delta\mathcal{C}_\circ$ for all trivial bands, and $\delta\mathcal{C}_{\circ,\nu_1} = \delta\mathcal{C}_{2\circ}$. This result is comparable to the one found in Ref. [35]. In that paper however, the proof was restricted to two-by-two matrices, whereas we provide a more general proof for a matrix with an arbitrary (but finite) number of bands. This is possible, because we can represent the matrix locally in an analytic form.

We are left with the calculation of the infinitesimal path enclosing the pole at $z = 0$. Since there are in general many exceptional points at finite $z$, corresponding to many pair creations of braid generators (see the conservation law argument from Sec. S2 S2.1), the topology of the spectrum on a closed path around $z = 0$ can be very complex and thus hard to treat. We may however perform the following trick. Referring to Sec. S2 S2.1, we first perform the transformation from the full $W(z)$ to $W_<(z)$. The idea is, that this transformation allows us to annihilate the exceptional points linked to the pole at $z \to \infty$, and thus making any braid generators associated with the $\infty$-pole vanish. At the same time, it will neither change the leading orders of the eigenspectrum nor of the eigenvectors in the vicinity of $z = 0$, such that the result for $\mathcal{Z}$ for a contour arbitrarily close to $z = 0$ remains the same. In a second step, we choose a sufficiently large, simple contour that encloses *all* remaining exceptional points at finite $z$ that are linked to the 0-pole, including the 0-pole itself. Now we know that the quantity $\mathcal{Z}$ for this path is necessarily $+1$: though the map $W_<(z) \to W_<(1/z)$ we can show that this contour is equivalent to the contour enclosing no exceptional points (thanks to the previous mapping from $W(z)$ to $W_<(z)$). We can thus conclude that the contour circumventing only the 0-pole results in a contribution $\mathcal{Z} = (-1)^{D_0}$, where $D_0$ is at the same time the number of braid generators $\sigma_n^{-1}$ that are associated to the 0-pole and (due to the previously elaborated conservation law) the number of exceptional points at finite $z$ for $W_<(z)$. This allows us to compute the number $\mathcal{Z}$ for an arbitrary closed contour.

We may now return to the original question, of the result for the number $\mathcal{Z}$ for the original matrix $W(z)$, for a simple closed contour around the unit circle $|z| \to 1$. Here, the result is

$$
\mathcal{Z} = (-1)^D \tag{S16}
$$

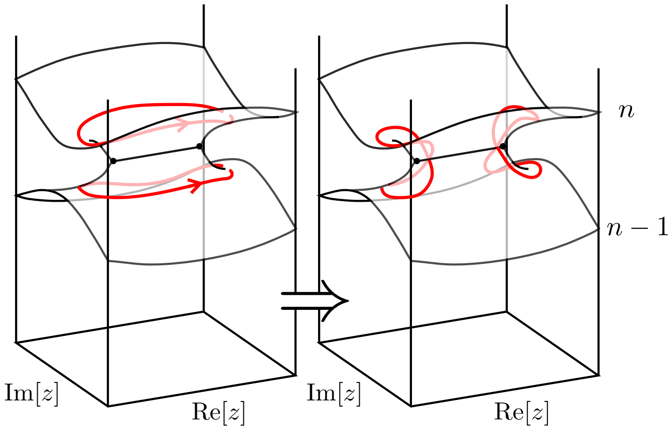


FIG. S4. Schematic depiction of a splitting of a large contour that may enclose several braid generators, here a pair of $\sigma_n$ and $\sigma_n^{-1}$. Only the subcontours that enclose an exceptional point (right image) contribute nontrivially to the topological number $\mathcal{Z}$. Note that the $z$-axis of the plot does here not correspond to the eigenspectrum. The $\sigma_n^{-1}$ braid operator, which can only occur at $z \to 0, \infty$ would actually lead to a divergent spectrum, which cannot be easily depicted. Instead we chose to plot a generic function, which is designed to depict only the connection of two braided bands, but not their actual values.

where $D$ is the number of braid generators enclosed by the contour. Since the contour includes $z = 0$, the integer number $D$ is composed of the number of exceptional points at finite $z$ with $|z| < 1$, plus $D_0$. In general, we see that $\mathcal{Z}$ can be represented as a $\mathbb{Z}_2$ group, where the nontrivial group operation corresponds to the process of an exceptional point (associated with a braid generator) leaving or entering the unit circle.

We may now in a final step relate the number $D$ to the periodicity of the eigenspectrum. For this purpose, we note that whatever the braiding topology of the spectrum for $|z| = 1$ is, the entering into or leaving of an exceptional point from the unit circle (associated with a single braid generator) can only either merge two bands $\nu_1$ and $\nu_2$, each with a certain periodicity $p_{\nu_1}$ and $p_{\nu_2}$, into a single band $\nu'$ with the sum of the two periodicities $p_{\nu'} = p_{\nu_1} + p_{\nu_2}$, or break down a single band $\nu$ with periodicity $p_\nu$ into two bands $\nu'_1$ and $\nu'_2$ and periodicities $p_{\nu'_1}$ and $p_{\nu'_2}$, such that likewise $p_{\nu'_1} + p_{\nu'_2} = p_\nu$. Overall, the quantity $\sum_\nu p_\nu$, which corresponds to the total number of eigenvalues $n_{\mathrm{tot}}$, remains constant, while the number of reduced bands, $\nu_{\mathrm{tot}} = \sum_\nu$, changes by either $+1$ or $-1$, depending on whether $D$ changes by $+1$ or $-1$. We remark that of course also bands with periodicity 1 can have a nontrivial braiding topology, however, those must necessarily contain an even number of braid generators, and hence provide a trivial contribution to the $\mathcal{Z}$ number. Eventually, while a trivial eigenspectrum results in $\mathcal{Z} = 1$, we can write $\mathcal{Z}$ for a generally nontrivial eigenspectrum as $\mathcal{Z} = (-1)^{n_{\mathrm{tot}} - \nu_{\mathrm{tot}}}$. With some algebra, we thus easily find that

$$\mathcal{Z} = \prod_{\widetilde{n}} (-1)^{p_{\widetilde{n}} - 1} , \tag{S17}$$

which is the result given in the main text in Eq. (30) .

## S3 Derivation of effective Hamiltonian for topological Josephson junction

Based on Eq. (31) in the main text, we can formulate an effective subgap Hamiltonian with a few simple steps. Assuming a constant $M$ for $0 < x < L$ (and $M = 0$ elsewhere), we can formulate a boundary condition for the wave function of the form $|\psi(L)\rangle = e^{e^{\frac{L}{v_F}[i\mu\sigma_z + M\tau_z\sigma_y]}}|\psi(0)\rangle$. Based on this, one can deduce the scattering matrices for incoming and outgoing electrons and holes, $S_{e,h}$, which are related through $S_h = -\sigma_z S_e^* \sigma_z$. Using Beenakker's formula [94], we find for the subgap energies the equation for the outgoing wave amplitudes $e^{i\theta(E)}|\psi\rangle_{\mathrm{out}} = S_A|\psi\rangle_{\mathrm{out}}$, with the scattering matrix including Andreev reflection $S_A = S_e e^{i\widehat{\phi}}\tau_+ + S_h e^{-i\widehat{\phi}}\tau_-$ where $\tau_\pm = (\tau_x + \pm i\tau_y)/2$, and the Andreev scattering phase $\cos[\theta(E)] = E/\Delta$. This equation can be rewritten as an effective Hamiltonian, by exploiting the unitarity of $S_A$, such that $e^{-i\theta(E)}|\psi\rangle_{\mathrm{out}} = S_A^\dagger|\psi\rangle_{\mathrm{out}}$. Taking the sum of these two equations, and getting rid of

the doubling of states in Eq. (31) we find

$$E|\psi\rangle = \frac{\Delta}{2}\begin{pmatrix} 0 & t_e\left[1+e^{i\phi}\right] \\ t_e^*\left[1+e^{-i\phi}\right] & 0 \end{pmatrix}|\psi\rangle\ , \tag{S18}$$

with the electron tunneling amplitude

$$t_e = \left[\cosh\left(\kappa\right) - i\frac{\mu}{\kappa}\sinh\left(\kappa\right)\right]^{-1}\ , \tag{S19}$$

with $\kappa = \sqrt{M^2-\mu^2}$. Thus we arrive at the effective Hamiltonian given in Eq. (32).

## S4 Extracting geometric phases from waiting times

In the main text, we provide with Eq. (39) an expression that directly links the geometric phase to quantities that can be extracted from the waiting times. We here provide the derivation for this expression. As in the main text, we focus on the specific measurement setup of a single level quantum dot coupled to a QPC. In this particular case, there are only detector clicks in one direction, say +, which means that only the waiting time correlations $g_{++}$ and $G_{++}$ are relevant. We take the Dyson-like equation for this correlator,

$$G_{++}\left(\tau\right) = g_{++}\left(\tau\right) + \int_0^\tau dt g_{++}\left(\tau-t\right)e^{i\chi(t)}G_{++}\left(t\right). \tag{S20}$$

We now perform the discretization of the time axis, such that the total measurement time $\tau$ is divided into $\tau = \Delta t_0 + \Delta t_1 + \ldots + \Delta t_M$. For each time interval $\Delta t_m$, where $m$ is integer and $0 \leq m \leq M$, we assign a constant counting field $\chi_m$. The inital counting field is chosen as $\chi_0 = 0$. The final value for $\chi$ has to be chosen according to the periodicity of the considered eigenvalue $\nu$, $\chi_M = 2\pi p_\nu$. We subsequently change to Laplace space for each small time interval, expressed through the operator $\mathcal{L}_M = \prod_{m=0}^M \int_0^\infty d\Delta t_m e^{-z\Delta t_m}$. Thus, we find for $G_{++}\left(z_0, z_1, \ldots\right) = \mathcal{L}_M G_{++}\left(\Delta t_0, \Delta t_1, \ldots\right)$, the equation

$$G_{++}^{(0,M)} = g_{++}^{(0,M)} + \sum_{m=0}^M e^{i\chi_m} g_{++}^{(m,M)} G_{++}^{(0,m)} \tag{S21}$$

where we used the notation $G_{++}^{(m,M)} = G_{++}\left(z_m, z_{m+1}, \ldots, z_M\right)$ and similarly for $g_{++}$. The free correlator is of the form

$$g_{++}\left(\tau\right) = g_{++,0}e^{l_0\tau} + g_{++,1}e^{l_1\tau} \tag{S22}$$

where again $l_{0,1}$ are the eigenvalues of $W_0$. We find for $m' > m$

$$g_{++}^{(m,M)} = g_{++,0}\prod_{m'=m}^M \frac{1}{z_{m'}-l_0} + g_{++,1}\prod_{m'=m}^M \frac{1}{z_{m'}-l_1}, \tag{S23}$$

where $g_{++}^{(m,m)} = g_{++}[z_m]$ is the ordinary Laplace transform of $g_{++}(\tau)$. We can now first reexpress Eq. (S21) into a recursive formula

$$G_{++}^{(0,n)} = \frac{g_{++}^{(0,n)} + \sum_{m=0}^{n-1} e^{i\chi_m} g_{++}^{(m,n)} G_{++}^{(0,m)}}{1 - e^{i\chi_n} g_{++}^{(n,n)}}. \tag{S24}$$

This can be solved formally as

$$G_{++}^{(0,M)} = \frac{1}{\prod_{m=0}^M \left[1 - e^{i\chi_m} g_{++}^{(m,m)}\right]} \prod_{m=1}^{M-1}\left[1 - e^{i\chi_m} g_{++}^{(m,m)} + \mathcal{K}_m\right] g_{++}^{(0,M)}\ , \tag{S25}$$

where the operator $\mathcal{K}_m$ is a “cutting” operator acting on $g_{++}$ as follows,

$$\mathcal{K}_{m_1} g_{++}^{(m,m')} = e^{i\chi_{m_1}} g_{++}^{(m,m_1)} g_{++}^{(m_1,m')} \tag{S26}$$

requiring $m < m_1 < m'$, whereas for all other $m$ and $m'$ it commutes with the correlator $g^{(m,m')}$. We finally perform the task of selecting a single eigenvalue $\nu$ from $G_{++}$, to extract the corresponding geometric phase $\mathcal{B}_\nu$. As mentioned in the main text, we do this through the operation

$$\mathcal{B}_\nu = \frac{1}{g_{++}[\lambda_\nu(0)]} \prod_{m=0}^{M} \lim_{z_m \to \lambda_\nu(\chi_m)} [z_m - \lambda_\nu(\chi_m)]\, G_{++}^{(0,M)}. \tag{S27}$$

Without loss of generality, we here choose $\nu = 0$. In a next important step, we can use the identity

$$(z_m - l_0)(z_m - l_1)\left(1 - e^{i\chi_m} g_{++}^{(m,m)}\right) = [z_m - \lambda_0(\chi_m)]\,[z_m - \lambda_1(\chi_m)] \tag{S28}$$

to show that Eq. (S27) reduces to

$$\mathcal{B}_0 = \frac{1}{g_{++}[\lambda_0(0)]} \prod_{m=0}^{M} \lim_{z_m \to \lambda_{\bar{0}}(\chi_m)} \frac{(z_m - l_0)(z_m - l_1)}{[z_m - \lambda_1(\chi_m)]} \prod_{m'=1}^{M-1} \mathcal{K}_{m'} g_{++}^{(0,M)}. \tag{S29}$$

Finally, with

$$\prod_{m=1}^{M-1} \mathcal{K}_m g_{++}^{(0,M)} = e^{i\chi_1} \dots e^{i\chi_{M-1}} g_{++}^{(0,1)} g_{++}^{(1,2)} \dots g_{++}^{(M-1,M)}, \tag{S30}$$

and some recasting, we arrive at Eq. (39) from the main text. Note that in order to compactify Eq. (39), we used the fact that we start from $\chi_0 = 0$, such that for a closed contour, $e^{i\chi_0} = e^{i\chi_M} = 1$. Thus, we can add a factor $e^{i\chi_M}$ without changing the expression.
